# Supplementary material for: Alleviating the Long-Tail Problem in Conversational Recommender Systems
Source: arXiv:2307.11650 source file (2023-07-21)
Supplement: Supplementary file 1 [file appendix.tex]

\section{Further Analysis}
Here, we perform further analysis on our proposed model.

\subsection{Performance Comparison w.r.t. the Amount of Training Data}
Learning the parameters of CRSs requires a considerable amount of training data.
However, in real-world applications, they are likely to suffer from the cold start problem caused by insufficient data, which may increase the risk of overfitting.
Fortunately, since our approach only needs to optimize a few parameters in the prompt and incorporates a prompt pre-training strategy, the overfitting risk can be reduced to some extend.
To validate this, we simulate a data sparsity scenario by using different proportions of the training data, and report the results of Recall@10 and Recall@50 on the \textsc{ReDial} dataset.

Figure~\ref{fig:few-shot} shows the evaluation results. 
As we can see, the performance of baseline models substantially drops with less available training data, while our method is consistently better than all the baseline models in all cases.
It indicates that our model is more capable of efficiently utilizing the training data.
%This observation implies that our proposed model has a higher training efficiency with the prompt learning strategies.
By reducing the number of trainable parameters and incorporating the pre-trained KG-enhanced prompt, the influence of the cold start problem can be alleviated.
Under the extreme sparsity level (\ie 20\%), we can see that our model still achieves a comparable performance with the best baseline that is trained with full data. It further indicates the effectiveness of our model in the cold start scenario.

\begin{figure}[t]
    \centering
    \includegraphics[width=0.49\linewidth]{few-shot_recall-10.pdf}
    \includegraphics[width=0.49\linewidth]{few-shot_recall-50.pdf}
    \caption{Performance comparison w.r.t. different amount of training data on \textsc{ReDial} dataset.}
    \label{fig:few-shot}
\end{figure}

\subsection{Parameter Tuning}

\begin{figure}[t]
    \centering
    \includegraphics[width=0.49\linewidth]{prompt_rec.pdf}
    \includegraphics[width=0.49\linewidth]{prompt_conv.pdf}
    \caption{Performance tuning of our model w.r.t the length of the soft tokens on the \textsc{ReDial} dataset.}
    \label{fig:tune}
\end{figure}
Our approach includes a few hyper-parameters to tune. 
Here, we report the results of tuning the length of the task-specific soft prompts for the recommendation and conversation tasks, respectively.
We conduct the analysis experiments on the \textsc{ReDial} dataset and show the performance change curves of the two tasks in Figure~\ref{fig:tune}.

For the recommendation task, we can see that our model achieves the best performance when the length of continuous prompt is set to 10. 
It indicates that short prompts are able to preserve the task-specific knowledge about the recommendation task. Instead, too long prompts (\ie 100) may increase the risk of overfitting and degrade the performance.
For the conversation task, we can also see that our model performs the best when the prompt length is set to 50, and either too short or too long prompts can degrade the performance. A possible reason is that too short prompts are hard to preserve sufficient task information, while too long ones may lead to overfitting.
